# Supplementary material for: Robust Iris Presentation Attack Detection Fusing 2D and 3D Information
Source: arXiv:2002.09137 source file (2020-08-05)
Supplement: Supplementary file 1 [file appendix.tex]

\section{Results of more experiments}
\subsection{More Experimental Results}
The performance of all available open source iris PAD methods when trained on Ciba Vision samples and tested on Johnson\&Johnson samples (including samples from both \textit{NDCLD'15} and \textit{NDIris3D}) is shown in Table~\ref{table:brand_ciba_jnj}. In Table~\ref{table:brand_jnj_ciba}, the experiment is repeated but the training and testing sets are flipped. 
% Test scenario  --- train cibavision (mixed old & new), test johnson johnson (mixed old & new)
\begin{table}
\begin{center}
\begin{tabular}{cccc}
\toprule
\multirow{2}{*}{Methods} & \multicolumn{3}{c}{Performance}\\ \cline{2-4}
 & Acc. (\%) & APCER (\%) & BPCER (\%)\\ %\hline
\midrule
OSPAD-3D & 85.77 & 15.15 & 13.33 \\ %\hline
OSPAD-2D & 58.05 & 83.43 & 1.39 \\ %\hline
DACNN & 80.76 & 19.45 & 37.97 \\ %\hline
SIDPAD & 66.67 & 65.63 & 1.76 \\ %\hline
RegionalPAD & 61.00 & 75.47 & 3.33 \\ %\hline
\bottomrule
\end{tabular}
\end{center}
\caption{Performance of all iris PAD methods when trained on Ciba Vision data and  tested on Johnson \& Johnson data.}
\label{table:brand_ciba_jnj} 
\end{table}

% Test scenario  --- train johnson johnson (mixed old & new), test cibavision (mixed old & new)
\begin{table}
\begin{center}
\begin{tabular}{cccc}
\toprule
\multirow{2}{*}{Methods} & \multicolumn{3}{c}{Performance}\\ \cline{2-4}
 & Acc. (\%) & APCER (\%) & BPCER (\%)\\ %\hline
\midrule
OSPAD-3D & 87.77 & 11.55 & 12.90 \\ %\hline
OSPAD-2D & 77.49 & 43.56 & 1.42 \\ %\hline
DACNN & 64.69 & 68.75 & 1.80 \\ %\hline
SIDPAD & 68.82 & 59.28 & 3.04 \\ %\hline
RegionalPAD & 94.05 & 5.59 & 5.12 \\ %\hline
\bottomrule
\end{tabular}
\end{center}
\caption{Performance of all iris PAD methods when trained on Johnson \& Johnson data and  tested on Ciba Vision data.}
\label{table:brand_jnj_ciba} 
\end{table}

The decision maps of OSPAD-fusion when trained on the \textit{NDCLD'15} subset and tested on the \textit{NDIris3D} (both LG4000 and AD100) are shown in Figure~\ref{fig:fusion_3D_vs_2D_newLG4000} and~\ref{fig:fusion_3D_vs_2D_newAD100}.

\begin{figure}
    \centering
    \includegraphics[width=0.48\textwidth]{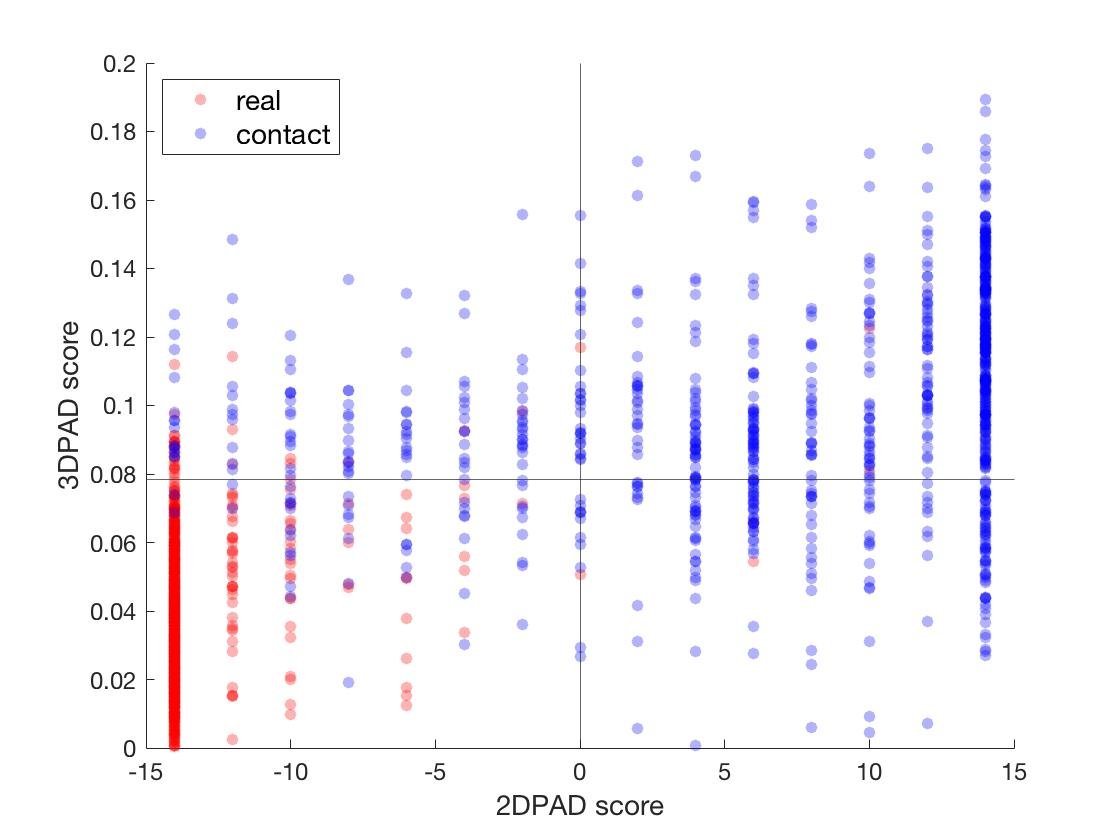}
    \caption{PAD score distribution of 3DPAD v.s. 2DPAD for the new LG4000 data.}
    \label{fig:fusion_3D_vs_2D_newLG4000}
\end{figure}

\begin{figure}
    \centering
    \includegraphics[width=0.48\textwidth]{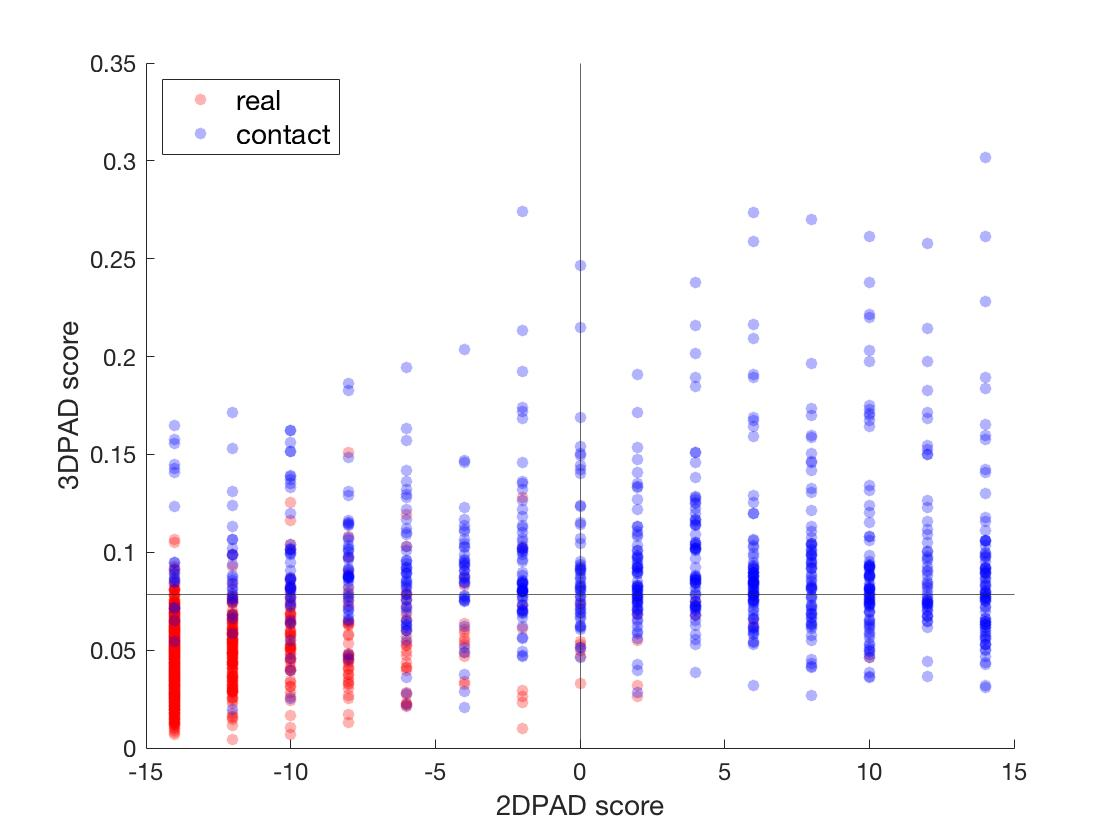}
    \caption{PAD score distribution of 3DPAD v.s. 2DPAD for the new AD100 data.}
    \label{fig:fusion_3D_vs_2D_newAD100}
\end{figure}

% \subsection{Camera Illuminant Angles}
% The angles of illuminant are briefly described here. For AD100, the left eye has a tilt angle of 115.887\degree
